# Supplementary material for: Crystal Structure and Magnetic Properties of the New Zn1.5Co1.5B7O13Br Boracite
Source: arXiv:1106.5446 source file (2011-06-27)
Supplement: Supplementary file 1 [file Suplementary_1.pdf]

# 'Crystal Structure and Magnetic Properties of the New $Zn_{1.5}Co_{1.5}B_7O_{13}Br$ Boracite'

**Roberto Escudero,[a]* Francisco Morales,[a] Marco Antonio Leyva-Ramirez,[b] J. Campa-Molina[c] and S. Ulloa-Godinez[c]**

[a]Instituto De Investigaciones en Materiales, Universidad Nacional Autónoma de México, Apartado Postal 70-360, 04510 México, D.F., MÉXICO, [b]Departamento de Química, Centro de Investigación y de Estudios Avanzados, del Instituto Politécnico Nacional, Apartado Postal 14-740, 07000 México, D.F., MÉXICO, and [c]C. Universitario de Ciencias Exactas e Ingenierías, Laboratorio de Materiales Avanzados, Departamento de Electrónica, Universidad de Guadalajara, Avenida Revolución # 1500, módulo O, 44840 Guadalajara, Jalisco, MÉXICO

Correspondence email: escu@servidor.unam.mx

New $Zn_{1.5}Co_{1.5}B_7O_{13}Br$ boracite crystals were grown by chemical transport reactions in quartz ampoules, at temperature of 1173 K. The crystal structure was characterized by X-Ray diffraction. The crystal presents an orthorhombic structure with space group $Pca2_1$, (No. 29). The determined cell parameters were: a = 8.5705 (3)Å, b = 8.5629 (3)Å, and c = 12.1198 (4)Å, and the cell volume, V = 889.45 (5)$Å^3$ with Z = 4. Magnetic properties in single crystals of the new boracite, were determinated. The Susceptibility-Temperature (χ - T ) behavior at different magnetic intensites was studied; χ(T) displays irreversibility below about 5 to 7 K, this disappears at high magnetic fields, about 5000 Oe. The inverse of the magnetic susceptibility $\chi^{-1}$(T) shows a Curie-Weiss characteristic with spin s = 3/2 and small orbital contribution, l. At low temperatures, below 10 K, χ(T) shows irreversibility that is strongle dependent on the applied magnetic field. This boracites is ferrimagnetic up to a maximum temperature about 16 K, as shows the coercive field. The reduccion of the irreversibility by the influence of the magnetic field, may be related to a metamagnetic phase transition.

## Experimental

### *Crystal data*

| | |
|---|---|
| $(Co{\cdot}Zn)_3B_7O_{13}Br$ | $V$ = 889.45 (5) $Å^3$ |
| $M_r$ = 550.03 | $Z$ = 4 |
| Orthorhombic, $Pca2_1$ | Mo $K\alpha$ radiation, λ = 0.71073 Å |
| $a$ = 8.5705 (3) Å | $\mu$ = 11.37 $mm^{-1}$ |
| $b$ = 8.5629 (3) Å | $T$ = 293 K |
| $c$ = 12.1198 (4) Å | 0.19 × 0.11 × 0.08 mm |

### *Data collection*

| | |
|---|---|
| KappaCCD diffractometer | 2027 independent reflections |
| Absorption correction: Multi-scan [c.f. r.h. blessing, acta cryst. (1995), a51, 33-38] | 1273 reflections with $I > 2\sigma(I)$ |
| $T_{min}$ = 0.186, $T_{max}$ = 0.273 | $R_{int}$ = 0.060 |
| 10425 measured reflections | |

*Refinement*

| | |
|---|---|
| $R[F^2 > 2\sigma(F^2)] = 0.033$ | 1 restraint |
| $wR(F^2) = 0.083$ | $\Delta\rho_{max} = 3.14$ e Å$^{-3}$ |
| $S = 1.00$ | $\Delta\rho_{min} = -3.02$ e Å$^{-3}$ |
| 2027 reflections | Absolute structure: Flack H D (1983), Acta Cryst. A39, 876-881 |
| 116 parameters | Flack parameter: 0.063 (18) |

Data collection: Collect (Bruker AXS BV, 1997-2004); cell refinement: *HKL SCALEPACK* (Otwinowski & Minor 1997); data reduction: *HKL DENZO* and *SCALEPACK* (Otwinowski & Minor 1997); program(s) used to solve structure: *SHELXS97* (Sheldrick, 2008); program(s) used to refine structure: *SHELXL97* (Sheldrick, 2008); molecular graphics: Diamond (Brandenburg, 1999); software used to prepare material for publication: *WinGX* publication routines (Farrugia, 1999).

## References


Blessing, R. H. (1995). Acta Cryst., A51, 33-38.

Blessing, R. H. (1987). Cryst. Rev. 1, 3-58.

Blessing, R. H. (1989). J. Appl. Cryst. 22, 396-397.

*COLLECT*: Nonius [or Hooft, R. W. W.] (1998). *COLLECT*. Nonius BV, Delft, The Netherlands.

*DENZO*/*SCALEPACK*: Otwinowski, Z. & Minor, W. (1997). Methods in Enzymology, Vol. 276, Macromolecular Crystallography, Part A, edited by C. W. Carter Jr & R. M. Sweet, pp. 307-326. New York: Academic Press.

*DIAMOND*: Brandenburg, K. [or Brandenburg, K. & Putz, H., or Brandenburg, K. & Berndt, M.] (1999). *DIAMOND*. Crystal Impact GbR, Bonn, Germany.

*EVALCCD*: Duisenberg, A. J. M., Kroon-Batenburg, L. M. J. & Schreurs, A. M. M. (2003). J. Appl. Cryst. 36, 220-229.

*PLATON*: Spek, A. L. (2003). J. Appl. Cryst. 36, 7-13.

*SADABS*: Bruker (2001). Bruker AXS Inc., Madison, Wisconsin, USA.

*SHELX* Sheldrick, G. M. (2008). Acta Cryst. A64, 112-122.

# supplementary materials

# 'Crystal Structure and Magnetic Properties of the New $Zn_{1.5}Co_{1.5}B_7O_{13}Br$ Boracite'

**Roberto Escudero,* Francisco Morales, Marco Antonio Leyva-Ramirez, J. Campa-Molina and S. Ulloa-Godinez**

## (re03c)

### *Crystal data*

| | |
|---|---|
| $(Co{\cdot}Zn)_3B_7O_{13}Br$ | $F(000) = 1038$ |
| $M_r = 550.03$ | $D_x = 4.107$ Mg m$^{-3}$ |
| Orthorhombic, $Pca2_1$ | Mo $K\alpha$ radiation, $\lambda = 0.71073$ Å |
| Hall symbol: P 2c -2ac | Cell parameters from 300 reflections |
| $a = 8.5705$ (3) Å | $\theta = 1$–14° |
| $b = 8.5629$ (3) Å | $\mu = 11.37$ mm$^{-1}$ |
| $c = 12.1198$ (4) Å | $T = 293$ K |
| $V = 889.45$ (5) Å$^3$ | Block, Purple |
| $Z = 4$ | 0.19 × 0.11 × 0.08 mm |

### *Data collection*

| | |
|---|---|
| KappaCCD diffractometer | 2027 independent reflections |
| Radiation source: Enraf Nonius FR590 | 1273 reflections with $I > 2\sigma(I)$ |
| graphite | $R_{int} = 0.060$ |
| Detector resolution: 9 pixels mm$^{-1}$ | $\theta_{max} = 27.4°$, $\theta_{min} = 2.9°$ |
| CCD rotation images, thick slices scans | $h = -9\rightarrow10$ |
| Absorption correction: Multi-scan [c.f. r.h. blessing, acta cryst. (1995), a51, 33-38] | $k = -11\rightarrow11$ |
| $T_{min} = 0.186$, $T_{max} = 0.273$ | $l = -15\rightarrow13$ |
| 10425 measured reflections | |

### *Refinement*

| | |
|---|---|
| Refinement on $F^2$ | Secondary atom site location: Difference Fourier map |
| Least-squares matrix: Full | $w = 1/[\sigma^2(F_o^2) + (0.0319P)^2]$ where $P = (F_o^2 + 2F_c^2)/3$ |
| $R[F^2 > 2\sigma(F^2)] = 0.033$ | $(\Delta/\sigma)_{max} = 0.001$ |
| $wR(F^2) = 0.083$ | $\Delta\rho_{max} = 3.14$ e Å$^{-3}$ |
| $S = 1.00$ | $\Delta\rho_{min} = -3.02$ e Å$^{-3}$ |
| 2027 reflections | Extinction correction: *SHELXL*, $Fc^*=kFc[1+0.001xFc^2\lambda^3/\sin(2\theta)]^{-1/4}$ |
| 116 parameters | Extinction coefficient: 0.0054 (4) |
| 1 restraint | Absolute structure: Flack H D (1983), Acta Cryst. A39, 876-881 |
| Primary atom site location: Structure-invariant direct methods | Flack parameter: 0.063 (18) |

*Special details*

**Geometry**. All s.u.'s (except the s.u. in the dihedral angle between two l.s. planes) are estimated using the full covariance matrix. The cell s.u.'s are taken into account individually in the estimation of s.u.'s in distances, angles and torsion angles; correlations between s.u.'s in cell parameters are only used when they are defined by crystal symmetry. An approximate (isotropic) treatment of cell s.u.'s is used for estimating s.u.'s involving l.s. planes.

**Refinement**. Refinement of $F^2$ against ALL reflections. The weighted R-factor wR and goodness of fit S are based on $F^2$, conventional R-factors R are based on F, with F set to zero for negative $F^2$. The threshold expression of $F^2 > 2\sigma(F^2)$ is used only for calculating R-factors(gt) etc. and is not relevant to the choice of reflections for refinement. R-factors based on $F^2$ are statistically about twice as large as those based on F, and R- factors based on ALL data will be even larger, The refinament have a twin domain and was determiated by the Platon software.

*Fractional atomic coordinates and isotropic or equivalent isotropic displacement parameters (Å²)*

| | *x* | *y* | *z* | $U_{iso}$*/$U_{eq}$ | Occ. (<1) |
|---|---|---|---|---|---|
| Co1 | 0.243 (2) | 0.7517 (19) | 0.7657 (4) | 0.0062 (2) | 0.5 |
| Co2 | 0.5231 (5) | 0.4629 (6) | 0.5001 (15) | 0.0062 (2) | 0.5 |
| Co3 | 1.0230 (5) | 0.9634 (6) | 0.4964 (15) | 0.0062 (2) | 0.5 |
| Zn1 | 0.2394 (17) | 0.7469 (16) | 0.7807 (3) | 0.0062 (2) | 0.5 |
| Zn2 | 0.5043 (4) | 0.4805 (5) | 0.4996 (12) | 0.0062 (2) | 0.5 |
| Zn3 | 1.0039 (4) | 0.9797 (6) | 0.4977 (12) | 0.0062 (2) | 0.5 |
| B1 | 0.4994 (11) | 0.5043 (18) | 0.7497 (8) | 0.008 (3)* | |
| B2 | 0.7435 (7) | 0.7531 (17) | 0.5057 (10) | 0.0069 (16)* | |
| B3 | 0.4989 (12) | 0.9962 (18) | 0.7498 (9) | 0.010 (3)* | |
| B4 | 0.5466 (9) | 0.7479 (11) | 0.6506 (6) | 0.0134 (15)* | |
| B5 | 0.7548 (8) | 0.5983 (12) | 0.8301 (7) | 0.0063 (19)* | |
| B6 | 0.4069 (8) | 0.2510 (11) | 0.6785 (6) | 0.0106 (14)* | |
| B7 | 0.7540 (9) | 0.9023 (13) | 0.8301 (7) | 0.011 (2)* | |
| O1 | 0.7658 (6) | 0.7490 (8) | 0.7620 (5) | 0.0052 (10)* | |
| O2 | 0.4592 (5) | 0.6698 (6) | 0.7263 (4) | 0.0103 (10)* | |
| O3 | 0.6185 (5) | 0.6703 (6) | 0.5660 (4) | 0.0086 (10)* | |
| O4 | 0.5329 (5) | 0.1635 (6) | 0.7291 (4) | 0.0112 (11)* | |
| O5 | 0.6781 (6) | 0.6378 (6) | 0.9334 (4) | 0.0089 (10)* | |
| O6 | 0.8329 (6) | 1.0271 (6) | 0.7703 (4) | 0.0107 (10)* | |
| O7 | 0.8592 (5) | 0.8265 (6) | 0.5756 (4) | 0.0100 (10)* | |
| O8 | 0.6652 (6) | 0.4816 (6) | 0.7698 (4) | 0.0115 (11)* | |
| O9 | 0.6713 (6) | 0.8744 (6) | 0.4351 (4) | 0.0107 (10)* | |
| O10 | 0.4517 (6) | 0.4087 (6) | 0.6556 (4) | 0.0102 (11)* | |
| O11 | 0.5403 (6) | 0.9108 (6) | 0.6474 (4) | 0.0098 (10)* | |
| O12 | 0.4131 (6) | 0.4586 (6) | 0.8497 (4) | 0.0099 (10)* | |
| O13 | 0.5889 (6) | 0.9413 (5) | 0.8445 (4) | 0.0093 (10)* | |
| Br1 | 0.26449 (7) | 0.74967 (16) | 0.99254 (7) | 0.0138 (2) | |

*Atomic displacement parameters (Å²)*

| | $U^{11}$ | $U^{22}$ | $U^{33}$ | $U^{12}$ | $U^{13}$ | $U^{23}$ |
|---|---|---|---|---|---|---|
| Co1 | 0.0054 (6) | 0.0065 (7) | 0.0066 (3) | 0.0000 (3) | −0.0001 (14) | 0.0015 (13) |
| Co2 | 0.0054 (6) | 0.0065 (7) | 0.0066 (3) | 0.0000 (3) | −0.0001 (14) | 0.0015 (13) |
| Co3 | 0.0054 (6) | 0.0065 (7) | 0.0066 (3) | 0.0000 (3) | −0.0001 (14) | 0.0015 (13) |
| Zn1 | 0.0054 (6) | 0.0065 (7) | 0.0066 (3) | 0.0000 (3) | −0.0001 (14) | 0.0015 (13) |
| Zn2 | 0.0054 (6) | 0.0065 (7) | 0.0066 (3) | 0.0000 (3) | −0.0001 (14) | 0.0015 (13) |

| | | | | | | |
|---|---|---|---|---|---|---|
| Zn3 | 0.0054 (6) | 0.0065 (7) | 0.0066 (3) | 0.0000 (3) | −0.0001 (14) | 0.0015 (13) |
| Br1 | 0.0147 (3) | 0.0131 (3) | 0.0136 (4) | 0.0001 (3) | −0.0003 (4) | 0.0003 (4) |

*Geometric parameters (Å, º)*

| | | | |
|---|---|---|---|
| Co1—O4$^{i}$ | 1.99 (2) | B4—O2 | 1.360 (9) |
| Co1—O2 | 2.04 (2) | B4—O3 | 1.368 (9) |
| Co1—O6$^{ii}$ | 2.047 (12) | B4—O11 | 1.397 (10) |
| Co1—O8$^{i}$ | 2.106 (13) | B5—O8 | 1.456 (10) |
| Co1—Br1 | 2.756 (5) | B5—O5 | 1.454 (9) |
| Co2—O12$^{iii}$ | 2.017 (18) | B5—O12$^{vii}$ | 1.462 (9) |
| Co2—O10 | 2.035 (18) | B5—O1 | 1.535 (11) |
| Co2—O5$^{iii}$ | 2.091 (7) | B6—O10 | 1.432 (11) |
| Co2—O3 | 2.112 (7) | B6—O4 | 1.450 (9) |
| Co2—Br1$^{iii}$ | 2.576 (3) | B6—O7$^{i}$ | 1.471 (9) |
| Co3—O9$^{iv}$ | 2.024 (13) | B6—O1$^{i}$ | 1.577 (9) |
| Co3—O7 | 2.065 (14) | B7—O9$^{viii}$ | 1.444 (10) |
| Co3—O13$^{v}$ | 2.085 (15) | B7—O6 | 1.457 (11) |
| Co3—O11$^{iv}$ | 2.128 (14) | B7—O13 | 1.464 (9) |
| Co3—Br1$^{v}$ | 2.582 (3) | B7—O1 | 1.554 (12) |
| Zn1—O4$^{i}$ | 2.028 (17) | O1—B6$^{vii}$ | 1.577 (9) |
| Zn1—O8$^{i}$ | 2.061 (11) | O4—B3$^{ix}$ | 1.484 (16) |
| Zn1—O6$^{ii}$ | 2.098 (10) | O4—Co1$^{vii}$ | 1.99 (2) |
| Zn1—O2 | 2.103 (17) | O4—Zn1$^{vii}$ | 2.028 (18) |
| Zn1—Br1 | 2.576 (4) | O5—B2$^{viii}$ | 1.481 (13) |
| Zn2—O12$^{iii}$ | 2.017 (16) | O5—Zn2$^{x}$ | 2.028 (7) |
| Zn2—O5$^{iii}$ | 2.028 (7) | O5—Co2$^{x}$ | 2.091 (7) |
| Zn2—O10 | 2.038 (16) | O6—B3$^{iv}$ | 1.458 (11) |
| Zn2—O3 | 2.061 (6) | O6—Co1$^{iv}$ | 2.047 (12) |
| Zn2—Br1$^{iii}$ | 2.796 (2) | O6—Zn1$^{iv}$ | 2.098 (10) |
| Zn3—O7 | 2.038 (12) | O7—B6$^{vii}$ | 1.471 (9) |
| Zn3—O13$^{v}$ | 2.047 (13) | O8—Zn1$^{vii}$ | 2.061 (11) |
| Zn3—O9$^{iv}$ | 2.048 (11) | O8—Co1$^{vii}$ | 2.106 (13) |
| Zn3—O11$^{iv}$ | 2.066 (12) | O9—B7$^{v}$ | 1.444 (10) |
| Zn3—Br1$^{v}$ | 2.797 (3) | O9—Co3$^{ii}$ | 2.024 (13) |
| B1—O8 | 1.455 (11) | O9—Zn3$^{ii}$ | 2.048 (11) |
| B1—O10 | 1.463 (13) | O11—Zn3$^{ii}$ | 2.066 (12) |
| B1—O12 | 1.473 (11) | O11—Co3$^{ii}$ | 2.128 (14) |
| B1—O2 | 1.486 (15) | O12—B5$^{i}$ | 1.462 (9) |
| B2—O7 | 1.448 (12) | O12—Co2$^{x}$ | 2.017 (18) |
| B2—O3 | 1.479 (11) | O12—Zn2$^{x}$ | 2.017 (16) |
| B2—O5$^{v}$ | 1.481 (13) | O13—Zn3$^{viii}$ | 2.047 (13) |
| B2—O9 | 1.481 (14) | O13—Co3$^{viii}$ | 2.085 (15) |
| B3—O6$^{ii}$ | 1.458 (11) | Br1—Co2$^{x}$ | 2.576 (3) |
| B3—O13 | 1.460 (12) | Br1—Co3$^{viii}$ | 2.582 (3) |
| B3—O11 | 1.484 (12) | Br1—Zn2$^{x}$ | 2.796 (2) |
| B3—O4$^{vi}$ | 1.484 (16) | Br1—Zn3$^{viii}$ | 2.797 (3) |
| | | | |
| O4$^{i}$—Co1—O2 | 153.5 (3) | O6—B7—O13 | 109.9 (7) |
| O4$^{i}$—Co1—O6$^{ii}$ | 90.5 (8) | O9$^{viii}$—B7—O1 | 107.4 (7) |
| O2—Co1—O6$^{ii}$ | 88.9 (5) | O6—B7—O1 | 108.9 (6) |

| | | | |
|---|---|---|---|
| $O4^{i}$—Co1—$O8^{i}$ | 93.8 (5) | O13—B7—O1 | 108.6 (6) |
| O2—Co1—$O8^{i}$ | 88.1 (8) | B5—O1—B7 | 114.9 (6) |
| $O6^{ii}$—Co1—$O8^{i}$ | 175.2 (9) | B5—O1—$B6^{vii}$ | 113.1 (6) |
| $O4^{i}$—Co1—Br1 | 106.6 (6) | B7—O1—$B6^{vii}$ | 113.0 (6) |
| O2—Co1—Br1 | 99.8 (6) | B4—O2—B1 | 118.1 (6) |
| $O6^{ii}$—Co1—Br1 | 87.3 (3) | B4—O2—Co1 | 119.3 (5) |
| $O8^{i}$—Co1—Br1 | 89.5 (3) | B1—O2—Co1 | 119.6 (6) |
| $O12^{iii}$—Co2—O10 | 173.6 (3) | B4—O2—Zn1 | 123.4 (5) |
| $O12^{iii}$—Co2—$O5^{iii}$ | 90.7 (6) | B1—O2—Zn1 | 116.6 (5) |
| O10—Co2—$O5^{iii}$ | 90.9 (5) | Co1—O2—Zn1 | 4.9 (4) |
| $O12^{iii}$—Co2—O3 | 87.5 (5) | B4—O3—B2 | 117.7 (7) |
| O10—Co2—O3 | 87.6 (6) | B4—O3—Zn2 | 117.5 (5) |
| $O5^{iii}$—Co2—O3 | 144.3 (2) | B2—O3—Zn2 | 121.9 (7) |
| $O12^{iii}$—Co2—$Br1^{iii}$ | 90.7 (4) | B4—O3—Co2 | 121.2 (6) |
| O10—Co2—$Br1^{iii}$ | 94.8 (5) | B2—O3—Co2 | 119.8 (7) |
| $O5^{iii}$—Co2—$Br1^{iii}$ | 106.1 (2) | Zn2—O3—Co2 | 5.89 (15) |
| O3—Co2—$Br1^{iii}$ | 109.5 (2) | B6—O4—$B3^{ix}$ | 115.1 (6) |
| $O9^{iv}$—Co3—O7 | 170.7 (5) | B6—O4—$Co1^{vii}$ | 125.4 (6) |
| $O9^{iv}$—Co3—$O13^{v}$ | 91.5 (7) | $B3^{ix}$—O4—$Co1^{vii}$ | 119.5 (6) |
| O7—Co3—$O13^{v}$ | 92.6 (3) | B6—O4—$Zn1^{vii}$ | 125.8 (6) |
| $O9^{iv}$—Co3—$O11^{iv}$ | 85.7 (3) | $B3^{ix}$—O4—$Zn1^{vii}$ | 119.0 (5) |
| O7—Co3—$O11^{iv}$ | 86.3 (7) | $Co1^{vii}$—O4—$Zn1^{vii}$ | 5.3 (3) |
| $O13^{v}$—Co3—$O11^{iv}$ | 146.8 (3) | B5—O5—$B2^{viii}$ | 117.3 (6) |
| $O9^{iv}$—Co3—$Br1^{v}$ | 92.1 (3) | B5—O5—$Zn2^{x}$ | 125.0 (6) |
| O7—Co3—$Br1^{v}$ | 94.9 (4) | $B2^{viii}$—O5—$Zn2^{x}$ | 116.7 (7) |
| $O13^{v}$—Co3—$Br1^{v}$ | 104.1 (4) | B5—O5—$Co2^{x}$ | 127.6 (6) |
| $O11^{iv}$—Co3—$Br1^{v}$ | 109.0 (5) | $B2^{viii}$—O5—$Co2^{x}$ | 114.9 (7) |
| $O4^{i}$—Zn1—$O8^{i}$ | 94.0 (4) | $Zn2^{x}$—O5—$Co2^{x}$ | 5.89 (14) |
| $O4^{i}$—Zn1—$O6^{ii}$ | 88.0 (7) | B7—O6—$B3^{iv}$ | 115.9 (7) |
| $O8^{i}$—Zn1—$O6^{ii}$ | 171.6 (6) | B7—O6—$Co1^{iv}$ | 121.1 (7) |
| $O4^{i}$—Zn1—O2 | 143.5 (3) | $B3^{iv}$—O6—$Co1^{iv}$ | 119.3 (9) |
| $O8^{i}$—Zn1—O2 | 87.6 (7) | B7—O6—$Zn1^{iv}$ | 117.9 (6) |
| $O6^{ii}$—Zn1—O2 | 85.9 (4) | $B3^{iv}$—O6—$Zn1^{iv}$ | 120.6 (8) |
| $O4^{i}$—Zn1—Br1 | 112.1 (6) | $Co1^{iv}$—O6—$Zn1^{iv}$ | 5.0 (3) |
| $O8^{i}$—Zn1—Br1 | 95.6 (3) | B2—O7—$B6^{vii}$ | 119.4 (7) |
| $O6^{ii}$—Zn1—Br1 | 91.1 (3) | B2—O7—Zn3 | 115.2 (7) |
| O2—Zn1—Br1 | 103.9 (5) | $B6^{vii}$—O7—Zn3 | 120.9 (5) |
| $O12^{iii}$—Zn2—$O5^{iii}$ | 92.5 (6) | B2—O7—Co3 | 116.1 (7) |
| $O12^{iii}$—Zn2—O10 | 172.0 (3) | $B6^{vii}$—O7—Co3 | 117.4 (5) |
| $O5^{iii}$—Zn2—O10 | 92.6 (4) | Zn3—O7—Co3 | 5.98 (15) |
| $O12^{iii}$—Zn2—O3 | 88.9 (4) | B5—O8—B1 | 120.5 (7) |
| $O5^{iii}$—Zn2—O3 | 156.1 (2) | B5—O8—$Zn1^{vii}$ | 117.2 (6) |
| O10—Zn2—O3 | 88.9 (5) | B1—O8—$Zn1^{vii}$ | 116.0 (8) |
| $O12^{iii}$—Zn2—$Br1^{iii}$ | 84.6 (3) | B5—O8—$Co1^{vii}$ | 119.8 (6) |
| $O5^{iii}$—Zn2—$Br1^{iii}$ | 100.5 (2) | B1—O8—$Co1^{vii}$ | 115.5 (9) |
| O10—Zn2—$Br1^{iii}$ | 88.4 (3) | $Zn1^{vii}$—O8—$Co1^{vii}$ | 5.1 (3) |
| O3—Zn2—$Br1^{iii}$ | 103.38 (18) | $B7^{v}$—O9—B2 | 116.1 (6) |
| O7—Zn3—$O13^{v}$ | 94.6 (3) | $B7^{v}$—O9—$Co3^{ii}$ | 119.2 (6) |
| O7—Zn3—$O9^{iv}$ | 172.3 (6) | B2—O9—$Co3^{ii}$ | 122.1 (7) |
| $O13^{v}$—Zn3—$O9^{iv}$ | 92.0 (7) | $B7^{v}$—O9—$Zn3^{ii}$ | 122.4 (6) |
| O7—Zn3—$O11^{iv}$ | 88.7 (6) | B2—O9—$Zn3^{ii}$ | 120.4 (6) |
| $O13^{v}$—Zn3—$O11^{iv}$ | 158.2 (3) | $Co3^{ii}$—O9—$Zn3^{ii}$ | 6.04 (14) |

| | | | |
|---|---|---|---|
| $O9^{iv}—Zn3—O11^{iv}$ | 86.7 (2) | B6—O10—B1 | 116.8 (6) |
| $O7—Zn3—Br1^{v}$ | 89.4 (3) | B6—O10—Zn2 | 121.6 (4) |
| $O13^{v}—Zn3—Br1^{v}$ | 98.2 (3) | B1—O10—Zn2 | 119.5 (6) |
| $O9^{iv}—Zn3—Br1^{v}$ | 85.7 (2) | B6—O10—Co2 | 118.4 (4) |
| $O11^{iv}—Zn3—Br1^{v}$ | 103.4 (4) | B1—O10—Co2 | 120.7 (6) |
| O8—B1—O10 | 109.2 (9) | Zn2—O10—Co2 | 6.20 (14) |
| O8—B1—O12 | 108.5 (7) | B4—O11—B3 | 118.5 (7) |
| O10—B1—O12 | 110.7 (8) | $B4—O11—Zn3^{ii}$ | 118.9 (5) |
| O8—B1—O2 | 112.7 (9) | $B3—O11—Zn3^{ii}$ | 118.4 (7) |
| O10—B1—O2 | 108.6 (7) | $B4—O11—Co3^{ii}$ | 122.2 (5) |
| O12—B1—O2 | 107.1 (9) | $B3—O11—Co3^{ii}$ | 117.0 (7) |
| O7—B2—O3 | 114.5 (9) | $Zn3^{ii}—O11—Co3^{ii}$ | 5.6 (2) |
| $O7—B2—O5^{v}$ | 109.0 (5) | $B5^{i}—O12—B1$ | 114.9 (6) |
| $O3—B2—O5^{v}$ | 107.6 (9) | $B5^{i}—O12—Co2^{x}$ | 120.7 (4) |
| O7—B2—O9 | 108.7 (9) | $B1—O12—Co2^{x}$ | 121.3 (6) |
| O3—B2—O9 | 108.6 (5) | $B5^{i}—O12—Zn2^{x}$ | 124.0 (5) |
| $O5^{v}—B2—O9$ | 108.4 (9) | $B1—O12—Zn2^{x}$ | 119.8 (5) |
| $O6^{ii}—B3—O13$ | 109.8 (8) | $Co2^{x}—O12—Zn2^{x}$ | 6.26 (14) |
| $O6^{ii}—B3—O11$ | 108.0 (8) | B3—O13—B7 | 119.4 (6) |
| O13—B3—O11 | 111.9 (9) | $B3—O13—Zn3^{viii}$ | 117.1 (6) |
| $O6^{ii}—B3—O4^{vi}$ | 110.6 (9) | $B7—O13—Zn3^{viii}$ | 121.3 (5) |
| $O13—B3—O4^{vi}$ | 109.9 (8) | $B3—O13—Co3^{viii}$ | 114.9 (6) |
| $O11—B3—O4^{vi}$ | 106.7 (8) | $B7—O13—Co3^{viii}$ | 124.8 (6) |
| O2—B4—O3 | 121.0 (7) | $Zn3^{viii}—O13—Co3^{viii}$ | 5.9 (2) |
| O2—B4—O11 | 119.3 (6) | $Co2^{x}—Br1—Zn1$ | 95.04 (16) |
| O3—B4—O11 | 118.8 (6) | $Co2^{x}—Br1—Co3^{viii}$ | 90.1 (3) |
| O8—B5—O5 | 110.7 (6) | $Zn1—Br1—Co3^{viii}$ | 94.8 (4) |
| $O8—B5—O12^{vii}$ | 110.0 (7) | $Co2^{x}—Br1—Co1$ | 95.0 (8) |
| $O5—B5—O12^{vii}$ | 110.9 (6) | Zn1—Br1—Co1 | 1.3 (3) |
| O8—B5—O1 | 109.9 (6) | $Co3^{viii}—Br1—Co1$ | 93.5 (4) |
| O5—B5—O1 | 107.2 (7) | $Co2^{x}—Br1—Zn2^{x}$ | 0.3 (5) |
| $O12^{vii}—B5—O1$ | 108.1 (5) | $Zn1—Br1—Zn2^{x}$ | 94.8 (7) |
| O10—B6—O4 | 111.7 (6) | $Co3^{viii}—Br1—Zn2^{x}$ | 89.95 (11) |
| $O10—B6—O7^{i}$ | 109.6 (5) | $Co1—Br1—Zn2^{x}$ | 94.7 (2) |
| $O4—B6—O7^{i}$ | 109.4 (6) | $Co2^{x}—Br1—Zn3^{viii}$ | 89.75 (11) |
| $O10—B6—O1^{i}$ | 109.3 (6) | $Zn1—Br1—Zn3^{viii}$ | 95.0 (4) |
| $O4—B6—O1^{i}$ | 107.5 (5) | $Co3^{viii}—Br1—Zn3^{viii}$ | 0.4 (6) |
| $O7^{i}—B6—O1^{i}$ | 109.3 (5) | $Co1—Br1—Zn3^{viii}$ | 93.8 (3) |
| $O9^{viii}—B7—O6$ | 110.7 (6) | $Zn2^{x}—Br1—Zn3^{viii}$ | 89.6 (2) |
| $O9^{viii}—B7—O13$ | 111.2 (6) | | |

Symmetry codes: (i) $x-1/2$, $-y+1$, $z$; (ii) $x-1/2$, $-y+2$, $z$; (iii) $-x+1$, $-y+1$, $z-1/2$; (iv) $x+1/2$, $-y+2$, $z$; (v) $-x+3/2$, $y$, $z-1/2$; (vi) $x$, $y+1$, $z$; (vii) $x+1/2$, $-y+1$, $z$; (viii) $-x+3/2$, $y$, $z+1/2$; (ix) $x$, $y-1$, $z$; (x) $-x+1$, $-y+1$, $z+1/2$.
