# Supplementary material for: Crystal Structure and Magnetic Properties of the New Zn1.5Co1.5B7O13Br Boracite
Source: arXiv:1106.5446 source file (2011-06-27)
Supplement: Supplementary file 2 [file suplementary2.pdf]

# 'Crystal Structure and Magnetic Properties of the New $\text{Zn}_{1.5}\text{Co}_{1.5}\text{B}_7\text{O}_{13}\text{Br}$ Boracite'

Roberto Escudero,<sup>a\*</sup> Francisco Morales,<sup>a</sup> Marco Antonio Leyva-Ramirez,<sup>b</sup> J. Campa-Molina<sup>c</sup> and S. Ulloa-Godinez<sup>c</sup>

<sup>a</sup>Instituto De Investigaciones en Materiales, Universidad Nacional Autónoma de México, Apartado Postal 70-360, 04510 México, D.F., MÉXICO, <sup>b</sup>Departamento de Química, Centro de Investigación y de Estudios Avanzados, del Instituto Politécnico Nacional, Apartado Postal 14-740, 07000 México, D.F., MÉXICO, and <sup>c</sup>C. Universitario de Ciencias Exactas e Ingenierías, Laboratorio de Materiales Avanzados, Departamento de Electrónica, Universidad de Guadalajara, Avenida Revolución # 1500, módulo O, 44840 Guadalajara, Jalisco, MÉXICO

Correspondence email: escu@servidor.unam.mx

New  $\text{Zn}_{1.5}\text{Co}_{1.5}\text{B}_7\text{O}_{13}\text{Br}$  boracite crystals were grown by chemical transport reactions in quartz ampoules, at temperature of 1173 K. The crystal structure was characterized by X-Ray diffraction. The crystal presents an orthorhombic structure with space group  $\text{Pca}2_1$ , (No. 29). The determined cell parameters were:  $a = 8.5705(3)\text{Å}$ ,  $b = 8.5629(3)\text{Å}$ , and  $c = 12.1198(4)\text{Å}$ , and the cell volume,  $V = 889.45(5)\text{Å}^3$  with  $Z = 4$ . Magnetic properties in single crystals of the new boracite, were determined. The Susceptibility-Temperature ( $\chi - T$ ) behavior at different magnetic intensities was studied;  $\chi(T)$  displays irreversibility below about 5 to 7 K, this disappears at high magnetic fields, about 5000 Oe. The inverse of the magnetic susceptibility  $\chi^{-1}(T)$  shows a Curie-Weiss characteristic with spin  $s = 3/2$  and small orbital contribution, 1. At low temperatures, below 10 K,  $\chi(T)$  shows irreversibility that is strongly dependent on the applied magnetic field. This boracite is ferrimagnetic up to a maximum temperature about 16 K, as shows the coercive field. The reduction of the irreversibility by the influence of the magnetic field, may be related to a metamagnetic phase transition.

## Experimental

### Crystal data

|                                                               |                                                     |
|---------------------------------------------------------------|-----------------------------------------------------|
| $(\text{Co}\cdot\text{Zn})_3\text{B}_7\text{O}_{13}\text{Br}$ | $V = 889.45(5)\text{Å}^3$                           |
| $M_r = 550.03$                                                | $Z = 4$                                             |
| Orthorhombic, $\text{Pca}2_1$                                 | Mo $K\alpha$ radiation, $\lambda = 0.71073\text{Å}$ |
| $a = 8.5705(3)\text{Å}$                                       | $\mu = 11.37\text{mm}^{-1}$                         |
| $b = 8.5629(3)\text{Å}$                                       | $T = 293\text{K}$                                   |
| $c = 12.1198(4)\text{Å}$                                      | $0.19 \times 0.11 \times 0.08\text{mm}$             |

### Data collection

|                                                                                        |                                        |
|----------------------------------------------------------------------------------------|----------------------------------------|
| KappaCCD diffractometer                                                                | 2027 independent reflections           |
| Absorption correction: Multi-scan [c.f. r.h. blessing, acta cryst. (1995), a51, 33-38] | 1273 reflections with $I > 2\sigma(I)$ |
| $T_{\min} = 0.186$ , $T_{\max} = 0.273$                                                | $R_{\text{int}} = 0.060$               |
| 10425 measured reflections                                                             |                                        |

## Refinement

|                                 |                                                                |
|---------------------------------|----------------------------------------------------------------|
| $R[F^2 > 2\sigma(F^2)] = 0.033$ | 1 restraint                                                    |
| $wR(F^2) = 0.083$               | $\Delta\rho_{\max} = 3.14 \text{ e } \text{\AA}^{-3}$          |
| $S = 1.00$                      | $\Delta\rho_{\min} = -3.02 \text{ e } \text{\AA}^{-3}$         |
| 2027 reflections                | Absolute structure: Flack H D (1983), Acta Cryst. A39, 876-881 |
| 116 parameters                  | Flack parameter: 0.063 (18)                                    |

Data collection: Collect (Bruker AXS BV, 1997-2004); cell refinement: *HKL SCALEPACK* (Otwinowski & Minor 1997); data reduction: *HKL DENZO* and *SCALEPACK* (Otwinowski & Minor 1997); program(s) used to solve structure: *SHELXS97* (Sheldrick, 2008); program(s) used to refine structure: *SHELXL97* (Sheldrick, 2008); molecular graphics: Diamond (Brandenburg, 1999); software used to prepare material for publication: *WinGX* publication routines (Farrugia, 1999).

## References

- Blessing, R. H. (1995). Acta Cryst., A51, 33-38.
- Blessing, R. H. (1987). Cryst. Rev. 1, 3-58.
- Blessing, R. H. (1989). J. Appl. Cryst. 22, 396-397.
- COLLECT*: Nonius [or Hooft, R. W. W.] (1998). *COLLECT*. Nonius BV, Delft, The Netherlands.
- DENZO/SCALEPACK*: Otwinowski, Z. & Minor, W. (1997). Methods in Enzymology, Vol. 276, Macromolecular Crystallography, Part A, edited by C. W. Carter Jr & R. M. Sweet, pp. 307-326. New York: Academic Press.
- DIAMOND*: Brandenburg, K. [or Brandenburg, K. & Putz, H., or Brandenburg, K. & Berndt, M.] (1999). *DIAMOND*. Crystal Impact GbR, Bonn, Germany.
- EVALCCD*: Duisenberg, A. J. M., Kroon-Batenburg, L. M. J. & Schreurs, A. M. M. (2003). J. Appl. Cryst. 36, 220-229.
- PLATON*: Spek, A. L. (2003). J. Appl. Cryst. 36, 7-13.
- SADABS*: Bruker (2001). Bruker AXS Inc., Madison, Wisconsin, USA.
- SHELX* Sheldrick, G. M. (2008). Acta Cryst. A64, 112-122.
